# Supplementary material for: On Principled Local Optimization Methods for Federated Learning
Source: arXiv:2401.13216 source file (2024-01-24)
Supplement: Supplementary file 1 [file pre_appendix.tex]

The appendices are structured as follows. 
% In \cref{sec:related_works}, we discuss the additional related literature of this work.
In \cref{sec:additional_expr}, we include additional experiments and detailed setups. 
In \cref{sec:background}, we provide the necessary backgrounds for our theoretical results. 
We prove two of our main results, namely \cref{thm:1:simplified,thm:2}, in \cref{sec:proof:thm:1,sec:proof:thm:2}, respectively.
The proof of \cref{thm:0} is sketched in \cref{sec:small_lr}.
